# Supplementary material for: Exploiting Correlations Between Contexts and Definitions with Multiple Definition Modeling
Source: arXiv:2305.14717 source file (2023-05-24)
Supplement: Supplementary file 1 [file Appendix.tex]

\newpage
\section{Example Appendix}
\label{sec:appendix}
\subsection{Error Analysis}
\label{error_analysis}

We listed some examples two main types errors in predicted definitions by MDM in Table \ref{error_analysis} including incomplete predicted definitions and word overlapping. Incomplete predicted definitions means that not all the gold definition will be predicted by BART+hyp+DL. For example, "hollered" contains three senses in gold definitions but BART+hyp+DL only gives one. However, we found there is no contexts in WordWiki test data containing a sense about "complain". Hence, the absent definitions may be caused by the lack of contexts. \par
Besides, we found an overlapping problem which the target word appears in the predictions. There are two possible reasons for these: 1) We did not force the decoder not predicting the word itself with a well-designed decoding strategy. 2) There are some definitions also containing the word itself. which we can see from the case "damson". We calculated the overlapping rate in our predictions is 7.71\% while the overlapping rate in references is 4.73\%. Hence, there is a chance that this issue is caused by the gold definitions in dataset. \par

\subsection{Hypernym Generation}

We also calculated ROUGE score and BERTScore for different auxiliary tasks for BART model. From Table \ref{hyp_score}, the task of BART+word is easier than the others since it achieved higher ROUGE and BERTScore. Besides, BART+syn is considerably easier than hypernym generation. So the ROUGE scores for BART+syn also outperforms BART+hyp. Actually, the metrics scores of BART+word, BART+syn and BART+hyp is not comparable because the testing data for the three decoder is different. However, evaluations on auxiliary tasks could allow us choose auxiliary tasks for BART according to their difficulty.

\subsection{Case Study on SDM task}
Here we list several cases from BART-SDM and BART-MDM-Easy on Oxford test data. And from which, we could discover that the quality of definitions produced by BART-MDM-Easy is superior than BART-SDM. BART-MDM-Easy could understand the sense in contexts better since the MDM pretraining has empowered the BART model with an ability to tell the difference and similarity between senses in different contexts.
\begin{table}[htp]
\centering
\scalebox{0.98}{
\begin{tabular}{@{}l|cccc@{}}
\toprule
\textbf{Model}          & \textbf{R1} & \textbf{R2} & \textbf{RL} & \textbf{BS} \\ \midrule
\textbf{BART+word} & 76.88       & 0.02        & 76.84       & 98.27       \\
\textbf{BART+syn}  & 48.89       & 6.94        & 48.51       & 98.32       \\
\textbf{BART+hyp}  & 33.14       & 9.57        & 32.69       & 98.06       \\ \bottomrule
\end{tabular}
}
\caption{This table presents the evaluation metrics on auxiliary rasks including generation of the word itself, synonym generation and hypernym generation. R1, R2, RL are ROUGE\_1, ROUGE\_2 and ROUGE\_L. BS refers to BERTScore.}
\label{hyp_score}
\end{table}

\begin{table*}[!h]
\centering
\scalebox{0.6}{
\begin{tabular}{@{}ll@{}}
\toprule[2pt]
\multicolumn{2}{c}{\textbf{Missing Definitions}}                                                                                     \\ \midrule
\textbf{WORD} & \textbf{hollered}                                                                                                             \\ \midrule
\textbf{CONTEXTS} &
  \begin{tabular}[c]{@{}l@{}}<w> hollered <w> well , that hollered " <unk> ho ! " makes for a pretty sweet pop hook , you have to admit \\ <sep> not satisfied with the results from the squibs his crew had brought for him , peckinpah became exasperated ; he finally hollered : " \\that 's not what i want ! that 's not what i want ! " he then grabbed a real revolver and fired it into a nearby wall \\ <sep> strom stepped out into the hallway and hollered after bavetta , \\" you 'll take another one of my fucking calls again , right , you motherfucker ? " strom was fined for the incident \\ <sep>  as we neared the channel , the navy men in the bow hollered to us to keep our heads down or we 'd get them blown off \\ <sep> {[} ... {]} over and over again , she subsumes her pop sensibilities to their arsenal of clattering beats , \\hollered raps and over @-@ fussy production \\ <sep> with its half @-@ mumbled , half @-@ hollered vocals , deliberate percussion and drone @-@ \\gone @-@ aggressive guitars , spiderland 's urgency is almost traumatic to swallow : despondency never tasted so real\end{tabular} \\ \midrule
\textbf{DEF}  & shout out <sep> utter a sudden loud cry <sep> complain                     \\ \midrule
\textbf{PRED} & make a high-pitched, screeching noise                                                                                \\ \midrule\midrule
\textbf{WORD} & \textbf{misinterpret}                                                                                                         \\ \midrule
\textbf{CONTEXTS} &
  \begin{tabular}[c]{@{}l@{}}<w> misinterpret <w> this angers the stonecutters , who misinterpret homer 's good intentions as going mad with power \\ <sep> rhinehart describes the est training as a form of participatory theatre , writing : " seeing the trainer as a master actor ... \\permits us to evaluate his acts and words more intelligently than if we misinterpret him as being a scholar or scientist giving a lecture \\ <sep> " on this topic , pewdiepie has claimed that it is disappointing when a large chunk of people misinterpret a component of his character ; he states , " \\if i mention on twitter that i find this or that kickstarter project cool , people immediately start to ask what economical interests i might have in it\\ .......\end{tabular} \\ \midrule
\textbf{DEF}  & interpret falsely <sep> interpret wrongly <sep> interpret in the wrong way \\
\textbf{PRED} & interpret in the wrong way                                                                                           \\ \midrule \midrule
\multicolumn{2}{c}{\textbf{Word Overlappings}}                                                                                       \\ \midrule
\textbf{WORD} & \textbf{sifters}                                                                                                              \\ \midrule
\textbf{CONTEXTS} &
  \begin{tabular}[c]{@{}l@{}}<w> sifters <w> manchester corporation attempted to remove the smell of putrefaction by attaching \\cinder @-@ sifters to their closets so that fine ash could be poured on top of the excrement \\ <sep> in march , a few guano sifters arrived to harvest and sell the guano of the nesting birds as fertilizer \\ <sep> lambourne included musings about these guano sifters in his work \\ <sep> lambourne left the island early in the winter of 1896 along with the first group of guano sifters\end{tabular} \\ \midrule
\textbf{DEF}  & a household sieve (as for flour)                                                                                     \\ \midrule
\textbf{PRED} & a worker who sifters plants (fruit or flowers or vegetables etc.)                                                    \\ \midrule\midrule
\textbf{WORD} & \textbf{damson}                                                                                                               \\ \midrule
\textbf{CONTEXTS} &
  \begin{tabular}[c]{@{}l@{}}<w> damson <w>  the good huswifes jewell gives recipes for making fruit tarts using fruits as varied as apple , peach , cherry , damson , pear , and mulberry \\ <sep>  in europe , it was known by various names during the nineteenth century when it was used as a medicine ;\\ these names included bitter ash , <unk> , mountain damson and stave @-@ wood \\ <sep> the recipe for tart de <unk> , a fish pie from the recipe collection forme of cury , \\includes a mix of figs , raisins , apples and pears with fish ( salmon , codling or haddock ) and pitted damson plums under the top crust\end{tabular} \\ \midrule
\textbf{DEF}  & dark purple plum of the damson tree                                                                                  \\ \midrule
\textbf{PRED} & pearl-like fruit of the damson tree                                                                                  \\ \bottomrule[2pt]
\end{tabular}
}
\caption{This table shows errors among definitions predicted by BART+hyp+DL on WordWiki test data.}
\label{error_analysis}
\end{table*}

% Please add the following required packages to your document preamble:
% \usepackage{booktabs}
\begin{table*}[htp]
\scalebox{0.6}{
\begin{tabular}{@{}lll@{}}
\toprule[2pt]
\multicolumn{3}{c}{\textbf{Example 1}}                                                                                                                     \\ \midrule
\multicolumn{1}{l|}{WORD}                & \multicolumn{2}{l}{\textbf{nail}}                                                                                        \\ \midrule
\multicolumn{1}{l|}{CONTEXTS}            & \multicolumn{2}{l}{he nailed down a spot at harvard}                                                            \\ \midrule
\multicolumn{1}{l|}{DEFINITION}          & \multicolumn{2}{l}{succeed in obtaining a position}                                                             \\ \midrule
\multicolumn{1}{l|}{BART-SDM}          & \multicolumn{2}{l}{lose ( a position or status ) by one's superior authority over the opposing}                 \\ \midrule
\multicolumn{1}{l|}{BART-MDM-Easy} & \multicolumn{2}{l}{succeed in obtaining something, especially a difficult or unappetizing one}                  \\ \midrule[1.5pt]
\multicolumn{3}{c}{\textbf{Example 2}}                                                                                                                              \\ \midrule
\multicolumn{1}{l|}{WORD}                & \multicolumn{2}{l}{\textbf{accent}}                                                                                      \\ \midrule
\multicolumn{1}{l|}{CONTEXTS} &
  \multicolumn{2}{l}{in both cases , cobalt blue was used to accent certain elements including the bells , the man 's shoes , shirt , and hat , and the cantons of the flags .} \\ \midrule
\multicolumn{1}{l|}{DEFINITION}          & \multicolumn{2}{l}{emphasize ( a particular feature )}                                                          \\ \midrule
\multicolumn{1}{l|}{BART-SDM}          & \multicolumn{2}{l}{put on ( a hat ) in order to mark the time it has been worn.}                                \\ \midrule
\multicolumn{1}{l|}{BART-MDM-Easy} &
  \multicolumn{2}{l}{make ( a quality ) more noticeable by adding extra detail or prominent elements to something else} \\ \midrule[1.5pt]
\multicolumn{3}{c}{\textbf{Example 3}}                                                                                                                              \\ \midrule
\multicolumn{1}{l|}{WORD}                & \multicolumn{2}{l}{\textbf{tale}}                                                                                        \\ \midrule
\multicolumn{1}{l|}{CONTEXTS} &
  \multicolumn{2}{l}{new research , published yesterday , suggests children 's love of contemporary fiction means classic tales are being left on the shelves .} \\ \midrule
\multicolumn{1}{l|}{DEFINITION}          & \multicolumn{2}{l}{a fictitious or true narrative or story , especially one that is imaginatively recounted}    \\ \midrule
\multicolumn{1}{l|}{BART-SDM}          & \multicolumn{2}{l}{a piece of fiction containing a story, typically one that is not meant for immediate use to} \\ \midrule
\multicolumn{1}{l|}{BART-MDM-Easy} & \multicolumn{2}{l}{a series of stories, typically light and exciting or appealing in some way ; a story}        \\ \bottomrule[2pt]
\end{tabular}
}
\caption{This table gives examples for the predictions of BART-SDM and BART-MDM-Easy respectively.}
\label{sdm_case_study}
\end{table*}

\begin{table*}[]
\centering
\scalebox{0.55}{
\begin{tabular}{@{}llll@{}}
\toprule
\multicolumn{4}{c}{\textbf{DEL 1}} \\ \midrule
\multicolumn{1}{l|}{\textbf{WORD}} &
  \multicolumn{1}{l|}{brink} &
  \multicolumn{1}{l|}{\textbf{WORD}} &
  humbleness \\ \midrule
\multicolumn{1}{l|}{\textbf{CONTEXT}} &
  \multicolumn{1}{l|}{\begin{tabular}[c]{@{}l@{}}w brink w at last he implored edgar to guide him to the \\ brink of a cliff so that he could throw himself off .\end{tabular}} &
  \multicolumn{1}{l|}{\textbf{CONTEXT}} &
  w humbleness w  not everyone regards humility as a virtue \\ \midrule
\multicolumn{1}{l|}{\textbf{DEFINITION}} &
  \multicolumn{1}{l|}{the extreme edge of land before a steep slope or a body or water} &
  \multicolumn{1}{l|}{\textbf{DEFINITION}} &
  a disposition to be humble ; a lack of false pride \\ \midrule
\multicolumn{1}{l|}{\textbf{SDM\_PRED}} &
  \multicolumn{1}{l|}{the point at which something is likely to happen} &
  \multicolumn{1}{l|}{\textbf{SDM\_PRED}} &
  regard as worthy or worthy of consideration \\ \midrule
\multicolumn{1}{l|}{\textbf{MDM\_PRED}} &
  \multicolumn{1}{l|}{the edge of something} &
  \multicolumn{1}{l|}{\textbf{MDM\_PRED}} &
  the quality of being humble \\ \midrule
\multicolumn{4}{c}{\textbf{DEL 2}} \\ \midrule
\multicolumn{1}{l|}{\textbf{WORD}} &
  \multicolumn{1}{l|}{placement} &
  \multicolumn{1}{l|}{\textbf{WORD}} &
  mope \\ \midrule
\multicolumn{1}{l|}{\textbf{CONTEXT}} &
  \multicolumn{1}{l|}{\begin{tabular}[c]{@{}l@{}}w placement w  traders in cleckheaton are being offered the help of \\ special-needs teenagers on work placements .  sep students would also \\ go on more work experience placements and local business people would \\ visit the school to discuss their experiences and give advice .\end{tabular}} &
  \multicolumn{1}{l|}{\textbf{CONTEXT}} &
  \begin{tabular}[c]{@{}l@{}}w mope w  everyone seemed to have a good time , even fiona , who was \\ apparently trying to get over having the mopes whenever she was not the \\ direct focus of albert 's attention .  sep  i moped around the house for \\ most of the weekend , wishing scott was with me .\end{tabular} \\ \midrule
\multicolumn{1}{l|}{\textbf{DEFINITION}} &
  \multicolumn{1}{l|}{\begin{tabular}[c]{@{}l@{}}the action of finding a home , job , or school for someone \\ sep the temporary posting of someone in a workplace to enable them to \\ gain work experience\end{tabular}} &
  \multicolumn{1}{l|}{\textbf{DEFINITION}} &
  \begin{tabular}[c]{@{}l@{}}low spirits ; depression sep  wander about listlessly and \\ aimlessly because of unhappiness or boredom\end{tabular} \\ \midrule
\multicolumn{1}{l|}{\textbf{SDM\_PRED}} &
  \multicolumn{1}{l|}{the action of sampling something sep the way in which something is arranged} &
  \multicolumn{1}{l|}{\textbf{SDM\_PRED}} &
  feel despondency sep an act of moping \\
\multicolumn{1}{l|}{\textbf{MDM\_PRED}} &
  \multicolumn{1}{l|}{a person's place of employment sep  a place for someone to do something} &
  \multicolumn{1}{l|}{\textbf{MDM\_PRED}} &
  a period of unhappiness or unhappiness sep  wander aimlessly \\ \bottomrule
\end{tabular}
}
\caption{This table listed generated definitions from BART-SDM and BART-MDM on incomplete datasets in Quantitative Analysis on Generated Multiple Definition.}
\label{tabel_case_for_del}
\end{table*}
